# Supplementary material for: S-NeRF: Neural Radiance Fields for Street Views
Source: arXiv:2303.00749 source file (2023-03-01)
Supplement: Supplementary file 1 [file supplementary.tex]

\documentclass{article}

\usepackage{iclr2023_conference,times}

\usepackage[utf8]{inputenc} % allow utf-8 input
\usepackage[T1]{fontenc}    % use 8-bit T1 fonts
\usepackage{hyperref}       % hyperlinks
\usepackage{url}            % simple URL typesetting
\usepackage{booktabs}       % professional-quality tables
\usepackage{amsfonts}       % blackboard math symbols
\usepackage{nicefrac}       % compact symbols for 1/2, etc.
\usepackage{microtype}      % microtypography
\usepackage{xcolor}         % colors
\usepackage{graphicx}
\usepackage{subfigure} 
\usepackage{float}
\usepackage{amsmath}
\usepackage{multirow}
\usepackage[permil]{overpic}
% new command

\iclrfinalcopy

% \author{Ziyang Xie\thanks{Equal contribution.},
% ~Junge Zhang$^*$,
% ~Wenye Li, 
% ~Feihu Zhang,
% ~Li Zhang\thanks{Corresponding author with School of Data Science, Fudan University (lizhangfd@fudan.edu.cn).}  \\
% \vspace{1mm}
% Fudan University \\
% \url{https://ziyang-xie.github.io/s-nerf}
% }

% \title{Supplementary Materials of ``S-NeRF: Neural Radiance Fields for Street Views''}

\begin{document}
\input{file/supp_tex.tex}
\bibliographystyle{iclr2023_conference}
\bibliography{iclr2023_conference}
\end{document}
